# Supplementary material for: VL-CheckList: Evaluating Pre-trained Vision-Language Models with Objects, Attributes and Relations
Source: arXiv:2207.00221 source file (2023-06-22)
Supplement: Supplementary file 1 [file appendix.tex]

We further provide additional dataset-level results and more visualization in the appendix here. 
